# Supplementary material for: Likelihood-Based Inference with Separable Correlation Matrices
Source: arXiv:1805.00318 ancillary file (2026-04-14)
Supplement: Supplementary file 1 [file ekvall_gray_suppl.pdf]

# Supplemental material for separable correlation and maximum likelihood

K. O. Ekvall<sup>\*1</sup> and B. R. Gray<sup>2</sup>

<sup>1</sup>School of Statistics, University of Minnesota

<sup>2</sup>U.S. Geological Survey, Upper Midwest Environmental Sciences Center

## Proofs

*Proof of Proposition 1.* Let  $\theta = (\beta, U, V, W)$ ,  $\theta' = (\beta', U', V', W')$ ,  $Y = (Y_1^T, \dots, Y_n^T)^T$ ,  $E(Y) = \mu(\theta) = X\beta$ , and  $\text{cov}(Y) = \Omega(\theta) = I_n \otimes \Sigma(\theta)$ . That  $g(\beta, U, V, W) = g(\beta', U', V', W')$  for Lebesgue-almost all  $y_1, \dots, y_n$  is the same as to say that  $Y$  has the same distribution under  $\theta$  and  $\theta'$ . Since normal distributions are characterized by their mean vector and covariance matrix, it suffices to show that  $\theta \neq \theta'$  implies  $\mu(\theta) \neq \mu(\theta')$  or  $\Omega(\theta) \neq \Omega(\theta')$ , the latter of which is clearly equivalent to  $\Sigma(\theta) \neq \Sigma(\theta')$ .

Suppose  $\beta \neq \beta'$ , then  $\mu(\theta) = X\beta \neq X\beta' = \mu(\theta')$  since  $X$  has full column rank by assumption. If instead  $W \neq W'$ , then  $\Sigma(\theta) = W(U \otimes V)W \neq W'(U' \otimes V')W' = \Sigma(\theta')$  since the diagonal elements of the left and right hand sides do not agree. This is so because the elements of  $W$  and  $W'$  are non-negative, so if they don't agree then their squares do not either. If  $W = W'$  but  $V \neq V'$ , then since  $W$  is invertible,  $W(U \otimes V)W = W'(U' \otimes V')W'$  if and only if  $U \otimes V = U' \otimes V'$ . But the upper  $r \times r$  block of the left hand side is  $V$  since  $U_{1,1} = 1$ , and the upper  $r \times r$  block of the right hand side is  $U'$  by the same argument. Thus,  $U \otimes V \neq U' \otimes V'$  and  $W(U \otimes V)W \neq W'(U' \otimes V')W'$ . Lastly, if  $W = W'$ ,  $V = V'$ , but

---

<sup>\*</sup>Corresponding author: [ekvall@umn.edu](mailto:ekvall@umn.edu)

$U \neq U'$ , then  $W(U \otimes V)W = W'(U' \otimes V')W'$  if and only if  $U \otimes V = U' \otimes V'$ , which is true if and only if  $U \otimes V = U' \otimes V$ , which in turn is true if and only if  $U \otimes I_r = U' \otimes I_r$ , where the last step follows from left-multiplying both sides by the invertible matrix  $I_c \otimes V^{-1}$ . Clearly  $U \neq U'$  implies  $U \otimes I_r \neq U' \otimes I_r$ , so we are done.  $\square$

*Proof of Proposition 2.* Existence is proved constructively. Pick arbitrary  $\mathbf{y} = (U, V, w_1, \dots, w_q) \in \mathbf{Y}$  and let  $\tilde{U} = (U \circ I_c)^{1/2}$  and  $\tilde{V} = (V \circ I_r)^{1/2}$ , where  $\circ$  denotes the Hadamard product. Let  $\bar{U} = \tilde{U}^{-1}U\tilde{U}^{-1} \in \mathbb{C}_{++}^c$  and  $\bar{V} = \tilde{V}^{-1}V\tilde{V}^{-1} \in \mathbb{C}_{++}^r$ . Then by standard properties of Kronecker products:

$$\begin{aligned}\Sigma &= W(U \otimes V)W \\ &= W(\tilde{U} \otimes \tilde{V})(\bar{U} \otimes \bar{V})(\tilde{U} \otimes \tilde{V})W\end{aligned}$$

where  $W(\tilde{U} \otimes \tilde{V}) = (\tilde{U} \otimes \tilde{V})W$  since diagonal matrices commute. Thus, upon taking  $\bar{w}_i$  to be the  $i$ th diagonal entry of  $W(\tilde{U} \otimes \tilde{V})$ ,  $\mathbf{x} = (\bar{U}, \bar{V}, \bar{w}_1, \dots, \bar{w}_q) \in \mathbf{X}$  and  $\Sigma(\mathbf{x}) = \Sigma(\mathbf{y})$  by construction. Uniqueness of  $\mathbf{x}$  is immediate from Proposition 1.  $\square$

*Proof of Proposition 3.* The proof idea is similar to that of Theorem 2 in ? which gives an equivalent result for the separable covariance model. ? provide the following sufficient conditions for existence of a maximum likelihood estimator for constrained covariance matrices using the multivariate normal likelihood: i) the residual covariance matrix  $S = n^{-1} \sum_{i=1}^n (y_i - \hat{\beta}^T x_i)(y_i - \hat{\beta}^T x_i)^T$  is non-singular, and ii) for an arbitrary convergent sequence  $\Sigma^k$  ( $k = 1, 2, \dots$ ) with separable correlation, it holds that either a)  $\Sigma^* = \lim_{k \rightarrow \infty} \Sigma_k$  is non-negative definite and singular, or b)  $\Sigma^*$  is positive definite and has separable correlation. The proof consists of checking conditions i) and ii).

Condition i) follows immediately from the fact that  $nS$  has Wishart distribution with  $n - p > q$  degrees of freedom, see for example ? and the references therein.

Condition ii) may be equivalently stated as follows: all matrices on the boundary of the set of covariance matrices with separable correlation are singular, non-negative definite matrices. Take an arbitrary converging sequence  $\Sigma_k$  ( $k = 1, 2, \dots$ ) and conformable vector  $v$ . Note that  $v^T \Sigma^k v \geq 0$  for all  $k$  and  $\Sigma^k$  converging to  $\Sigma^*$  imply  $v^T \Sigma^* v = \lim_{k \rightarrow \infty} v^T \Sigma^k v \geq 0$ . Thus, if the limit matrix is singular it is indeed non-negative definite. Suppose the limit

matrix is non-singular. Write  $U^k, V^k, W^k$  for the components in the separable correlation decomposition assumed to exist for  $\Sigma^k$  ( $k = 1, 2, \dots$ ). Since the sequence  $\Sigma^k$  converges, so do the sequences of corresponding diagonal entries. The diagonal entries are the squares of the elements in  $W^k$ , which are positive for every  $k$  and, thus, it must be that  $W^k$  converges to  $W^*$  for some standard deviation matrix  $W^*$ . This  $W^*$  is positive definite since the limiting matrix  $\Sigma^*$  is assumed non-singular. Moreover, by the arguments in the proof of Theorem 2 in ?,  $U^k \otimes V^k$  converges to a positive definite matrix  $R^*$  which admits the decomposition  $R^* = U^* \otimes V^*$  for some symmetric, positive definite  $U^*$  and  $V^*$ , which need not be correlation matrices. Now Proposition 2 finishes the proof.  $\square$

## A Model for Sample Means

The decision to model data from different years as independent reflects inspection of sample means; that dissolved oxygen is driven by flow, photosynthesis, respiration and other variables that themselves vary considerably within and among years; and that sampling sites are reselected annually, thereby precluding dependence among years at the sampling unit scale. Strata are defined geomorphically, while reaches denote navigation pools that are routinely sampled by the U.S. Army Corps of Engineers' Long Term Resource Monitoring Element.

Let  $Y_{i,j,k,l}$  denote the  $l$ th measurement in year  $i$ , area  $j$ , and season  $k$ . Assume that correlation between different measurements only depend on in which area and season those measurements are taken. For example, any two distinct measurements from the same area and season are assumed equally correlated. Mathematically,

$$\text{cov}(Y_{i,j,k,l}, Y_{i',j',k',l'}) = \begin{cases} 0, & \text{if } i \neq i' \\ \sigma_{j,k}^2, & \text{if } i = i', j = j', k = k', l = l' \\ \rho_{j,k;j',k'} \sqrt{\sigma_{j,k}^2 \sigma_{j',k'}^2}, & \text{otherwise,} \end{cases} \quad (1)$$

where  $\sigma_{j,k}^2$  is a variance parameter depending on season and location, and  $\rho_{j,k;j',k'}$  is the correlation between measurements from location-area combinations  $(j, k)$  and  $(j', k')$ .

The sample means we model are  $Y_{i,j,k} = n_{i,j,k}^{-1} \sum_{l=1}^{n_{i,j,k}} Y_{i,j,k,l}$ . Every year, each season-area combination is sampled between 8 – 82 times, so  $8 \leq n_{i,j,k} \leq 82$  for all  $i, j, k$ . The

average number of measurements on which the sample means are based,  $n_{i,j,k}$ , is 39.5. The response vector in our model is taken to be all the measurements from the same year,  $Y_i = [Y_{i,1,1}, \dots, Y_{i,3,16}]^T \in \mathbb{R}^{48}$  ( $i = 1, \dots, n$ ), since  $\# \text{seasons} \times \# \text{areas} = 3 \times 16 = 48$ . We have 21 independent observations (years) of that response vector.

The dependence structure assumed in (1) implies:

$$\text{cov}(Y_{i,j,k}, Y_{i',j',k'}) = \begin{cases} 0, & \text{if } i \neq i' \\ \sigma_{j,k}^2 [n_{i,j,k}^{-1} + (1 - n_{i,j,k}^{-1})\rho_{j,k}], & \text{if } i = i', j = j', k = k' \\ \sigma_{j,k,j',k'}, & \text{otherwise.} \end{cases}$$

The second term in the expression for variances of sample means,  $\kappa_{i,j,k} = [n_{i,j,k}^{-1} + (1 - n_{i,j,k}^{-1})\rho_{j,k}]$ , changes by years, which complicates modeling. This complication does not arise in applications where one is modeling raw data rather than sample means, or where  $n_{i,j,k}$  in fact does not depend on  $i$ . Treating the covariance matrix as constant in years in our data example is an approximation, which error depends on how much  $\kappa_{i,j,k}$  differs among years. Exploratory analysis of the full data indicates  $\rho_{j,k} \approx 0.5$  for all  $j, k$ . Using this estimate, we examined the ratio  $[\max_i \kappa_{i,j,k} - \min_i \kappa_{i,j,k}] / \bar{\kappa}_{j,k}$ , where  $\bar{\kappa}_{j,k}$  is the average  $\kappa$  for season  $k$  and location  $j$  over the  $n = 21$  years. The maximum such ratio was around 0.08, with only two being greater than 0.05. For 42/48 season-location combinations, the ratio was less than 0.02.

## Convergence diagnostics

For each setting in Table 1, 10000 datasets were generated from the separable correlation model, using the same configuration as in our other simulations. The model was then fit, using our algorithm, to each of these datasets. The maximum number of iterations was set to 1000 and the tolerance parameter  $\epsilon$  in our algorithm to  $10^{-10}$ .

Table 1: Convergence diagnostics

| $r$ | $c$ | $n$ | Conv. | Max  | $V$  | $U$  |
|-----|-----|-----|-------|------|------|------|
| 2   | 2   | 2   | 0.18  | 0.00 | 0.82 | 0.01 |
| 2   | 2   | 4   | 0.76  | 0.24 | 0.00 | 0.00 |
| 2   | 2   | 10  | 1.00  | 0.00 | 0.00 | 0.00 |
| 2   | 4   | 2   | 0.01  | 0.00 | 0.99 | 0.00 |
| 2   | 4   | 4   | 0.07  | 0.92 | 0.01 | 0.00 |
| 2   | 4   | 10  | 1.00  | 0.00 | 0.00 | 0.00 |
| 15  | 15  | 2   | 0.01  | 0.00 | 0.91 | 0.07 |
| 15  | 15  | 4   | 0.00  | 1.00 | 0.00 | 0.00 |
| 15  | 15  | 10  | 1.00  | 0.00 | 0.00 | 0.00 |

Columns 4 – 7 are proportions out of 10,000 simulated datasets in which the algorithm terminated because it converged, reached the maximum number of iterations, an update of  $V$  was singular, or an update of  $U$  was singular, respectively.

## Additional simulations

Table 2 shows simulation results similar to those of the lower panel of Table 1 of the main article. In these simulations,  $\beta = 0$ ,  $x_i = 1$  ( $i = 1, \dots, n$ ),  $U$  and  $V$  have all off-diagonal entries set to  $1/2$ , and  $W$  is diagonal with entries evenly spaced between 0.1 and 10. Qualitatively the findings are similar to those of Table 1 in the main article in that i) the separable covariance model does better in terms of spectral error when the sample size is small, ii) the separable correlation model does better when sample size is larger, and iii) the bootstrap based likelihood ratio test with  $H_0$  : separable correlation has near nominal size in all settings where it is applicable.

Table 2: Estimation error and test size

Data generated with separable correlation and compound symmetry

| $n$ | $r$ | $c$ | $err_{cor}$ | $err_{cov}$ | $err_{ur}$ | $rej_{cov}$ | $rej_{cov,b}$ | $rej_{cor}$ | $rej_{cor,b}$ |
|-----|-----|-----|-------------|-------------|------------|-------------|---------------|-------------|---------------|
| 10  | 5   | 5   | 20.16       | 17.68       | -          | 0.97        | 0.77          | -           | -             |
| 10  | 5   | 15  | 54.78       | 37.51       | -          | 0.98        | 0.13          | -           | -             |
| 10  | 15  | 15  | 107.76      | 75.05       | -          | 1.00        | 0.33          | -           | -             |
| 20  | 5   | 5   | 12.54       | 12.05       | -          | 1.00        | 1.00          | -           | -             |
| 20  | 5   | 15  | 29.79       | 25.25       | -          | 0.96        | 0.68          | -           | -             |
| 20  | 15  | 15  | 64.23       | 50.64       | -          | 1.00        | 0.91          | -           | -             |
| 160 | 5   | 5   | 4.25        | 6.45        | 7.85       | 1.00        | 1.00          | 0.24        | 0.05          |
| 160 | 5   | 15  | 9.82        | 9.96        | 21.27      | 1.00        | 1.00          | 1.00        | 0.05          |
| 160 | 15  | 15  | 21.12       | 20.47       | -          | 1.00        | 1.00          | -           | -             |
| 320 | 5   | 5   | 3.03        | 5.83        | 5.53       | 1.00        | 1.00          | 0.12        | 0.06          |
| 320 | 5   | 15  | 6.93        | 7.96        | 15.15      | 1.00        | 1.00          | 0.98        | 0.05          |
| 320 | 15  | 15  | 14.91       | 16.89       | 42.98      | 1.00        | 1.00          | 1.00        | 0.06          |

Columns labeled  $err$  show average spectral norm errors. Subscripts indicate separable correlation, separable covariance, and unrestricted estimators. Columns with label  $rej$  show empirical rejection rates. The subscripts indicate the null hypotheses covariance separability and correlation separability. A second subscript  $b$  indicates the parametric bootstrap was used.
